# Supplementary material for: Bounding the Complexity of Formally Verifying Neural Networks: A Geometric Approach
Source: arXiv:2012.11761 source file (2021-03-25)
Supplement: Supplementary file 1 [file appendix.tex]

% !TEX root = ./main.tex

\section{Appendix} % (fold)
\label{sec:appendix}

\begin{definition}[Input Replicator NN]
	\label{def:input_replicator}
	Let $n < m$ be two integers. An \textbf{input replicator NN of size} 
	$(n,m)$ is a single-layer NN with the following parameter list:
	\begin{equation}
		\Gamma_{n,m} \triangleq \big(
			\left(
				\left[
					\begin{smallmatrix}
						I_n \\
						\llbracket I_n \rrbracket_{n,\cdot} \\
						\vdots \\
						\llbracket I_n \rrbracket_{n,\cdot} 
					\end{smallmatrix}
				\right],
				\left[
					\begin{smallmatrix}
						0 \\
						0 \\
						\vdots \\
						0 
					\end{smallmatrix}
				\right]
			\right)
		\big)
	\end{equation}
	where $I_n$ represents the $(n \times n)$ identity matrix, and the 
	$n^\text{th}$ row thereof, $\llbracket I_n \rrbracket_{n,\cdot}$ is 
	repeated enough times so that $\text{Arch}(\Gamma_{n,m}) = ((n,m))$. That 
	is $\Gamma_{n,m}$ has $n$ inputs and $m > n$ outputs, with the final $m-n$ 
	outputs exact copies of the $n^\text{th}$ input.
\end{definition}
\begin{definition}[Two element $\min$ NN]
	\label{def:two_elem_min_nn}
	A two element $\min$ NN is given by parameter list
	\begin{equation}
		\Theta_{\min} \triangleq \Big(
		(
		\left[
			\begin{smallmatrix}
				-1 & -1 \\
				\hphantom{-}1 & \hphantom{-}1 \\
				\hphantom{-}1 & -1 \\
				-1 & \hphantom{-}1
			\end{smallmatrix}
		\right]
		,
		\left[
			\begin{smallmatrix}
				0 \\
				0 \\
				0 \\
				0
			\end{smallmatrix}
		\right]
		),
		(
		\left[
			\begin{smallmatrix}
				-\frac{1}{2} & \frac{1}{2} & -\frac{1}{2} & -\frac{1}{2}
			\end{smallmatrix}
		\right],
		\left[
			\begin{smallmatrix}
				0
			\end{smallmatrix}
		\right]
		)
		\Big).
	\end{equation}
	This network presents at its out the minimum value of its two inputs.
\end{definition}
\begin{definition}[Two element $\max$ NN]
	\label{def:two_elem_max_nn}
	A two element $\max$ NN is given by parameter list
	\begin{equation}
		\Theta_{\max} = \Big(
		(
		\left[
			\begin{smallmatrix}
				\hphantom{-}1 & \hphantom{-}1 \\
				-1 & -1 \\
				-1 & \hphantom{-}1 \\
				\hphantom{-}1 & -1
			\end{smallmatrix}
		\right],
		\left[
			\begin{smallmatrix}
				0 \\
				0 \\
				0 \\
				0
			\end{smallmatrix}
		\right]
		),
		(
		\left[
			\begin{smallmatrix}
				\frac{1}{2} & -\frac{1}{2} & \frac{1}{2} & \frac{1}{2}
			\end{smallmatrix}
		\right],
		\left[
			\begin{smallmatrix}
				0
			\end{smallmatrix}
		\right]
		)
		\Big)
	\end{equation}
	This network presents at its out the maximum value of its two inputs.
\end{definition}

\begin{definition}[Pairwise $\min$/$\max$ NNs]
	\label{def:pairwise_minmax_NN}
	A \textbf{pairwise }$\min$ \textbf{NN of size} $n$ is a NN defined by the 
	following parameter list:
	\begin{equation}
		\Theta^\text{min}_{n \div 2} \triangleq 
		(\Theta_{\min} \parallel \dots \parallel \Theta_{\min})
		\circ
		\Gamma_{n, 2 \cdot \lceil n/2 \rceil}
	\end{equation}
	where the parallel composition includes $\lceil n/2 \rceil$ copies of 
	$\Theta_{\min}$. Note that $\Theta^\text{min}_{n \div 2}$ has exactly 
	$\lceil n/2 \rceil$ outputs. Also note that $\Theta^\text{min}_{2 \div 2} = 
	\Theta_{\min}$.

	A \textbf{pairwise }$\max$ \textbf{NN of size} $n$ is defined as above, but 
	with $\min$ replaced by $\max$.
\end{definition}

\begin{definition}[$n$-element $\min$/$\max$ NNs]
	\label{def:n-element_minmax_NN_full}
	An $n$\textbf{-element $\min$ network} is defined by the following 
	parameter list:

	\begin{equation}
		\Theta_{\min_n} \triangleq
			\Theta^{\text{min}}_{2 \div 2} 
		\circ
			\Theta^{\text{min}}_{4 \div 2}
		\circ 
			\dots
		\circ
			\Theta^{\text{min}}_{\lceil n/2 \rceil \div 2}
		\circ
			\Theta^{\text{min}}_{n \div 2}.
	\end{equation}
	$\Theta_{\min_n}$ outputs minimum from among its $n$ inputs using a divide 
	and conquer approach.

	An $n$\textbf{-element $\max$ network}, denoted by $\Theta_{\max_n}$, is 
	defined as above, only with all occurrences of $\min$ replaced by $\max$. 
	Analogously, $\Theta_{\max_n}$ outputs the maximum element from among its 
	$n$ inputs. 
\end{definition}

% section discussion (end)
